# Supplementary material for: Experimental Studies of Top Quark Production
Source: arXiv:1606.02936 source file (2016-08-02)
Supplement: Supplementary file 1 [file appendix.tex]

%% LaTeX2e class for student theses
%% sections/apendix.tex
%% 
%% Karlsruhe Institute of Technology
%% Institute for Program Structures and Data Organization
%% Chair for Software Design and Quality (SDQ)
%%
%% Dr.-Ing. Erik Burger
%% burger@kit.edu
%%
%% Version 1.1, 2014-11-21

\iflanguage{english}
{\chapter{Appendix}}    % english style
{\chapter{Anhang}}      % german style
\label{chap:appendix}

%% -------------------
%% | Example content |
%% -------------------
\section{First Appendix Section}
\label{sec:appendix:FirstSection}
		
\setcounter{figure}{0}
		
\begin{figure} [ht]
  \centering
  \missingfigure{A figure}
  \caption{A figure}
  \label{fig:anotherfigure}
\end{figure}

\dots
%% ---------------------
%% | / Example content |
%% ---------------------
